# Supplementary material for: Seismic response of the Mars Curiosity Rover: Implications for future planetary seismology
Source: arXiv:1804.08720 source file (2018-04-23)
Supplement: Supplementary file 1 [file Supplementary_material_small.pdf]

Supplementary material for "Seismic response of the Mars Curiosity Rover: Implications for future planetary seismology"

The following figures show spectrograms for all 3 components of the reference and deck seismometers for the entire duration of the experiment. Timing information is given in universal coordinated time (UTC).

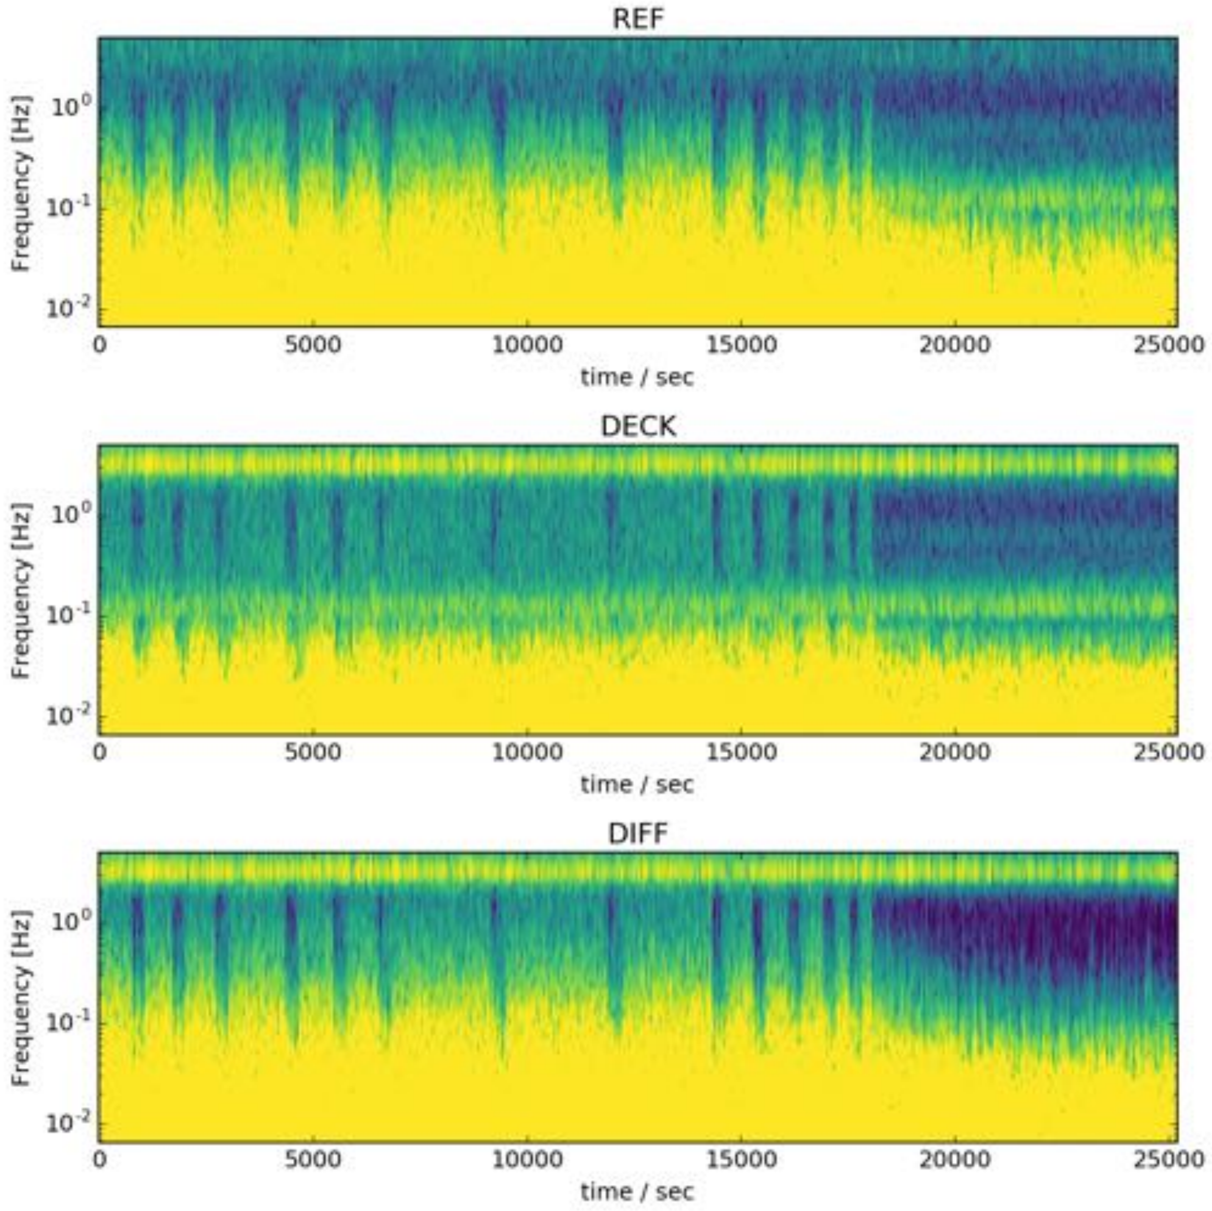


Figure S1: Spectrogram calculated as described in text for the east component of the reference (top) and deck (middle) seismometers, as well as the spectrogram of the difference between the components (bottom). This spectrogram covers the time period between 2017-10-06, 20:00 UTC and 2017-10-07 03:00 UTC.

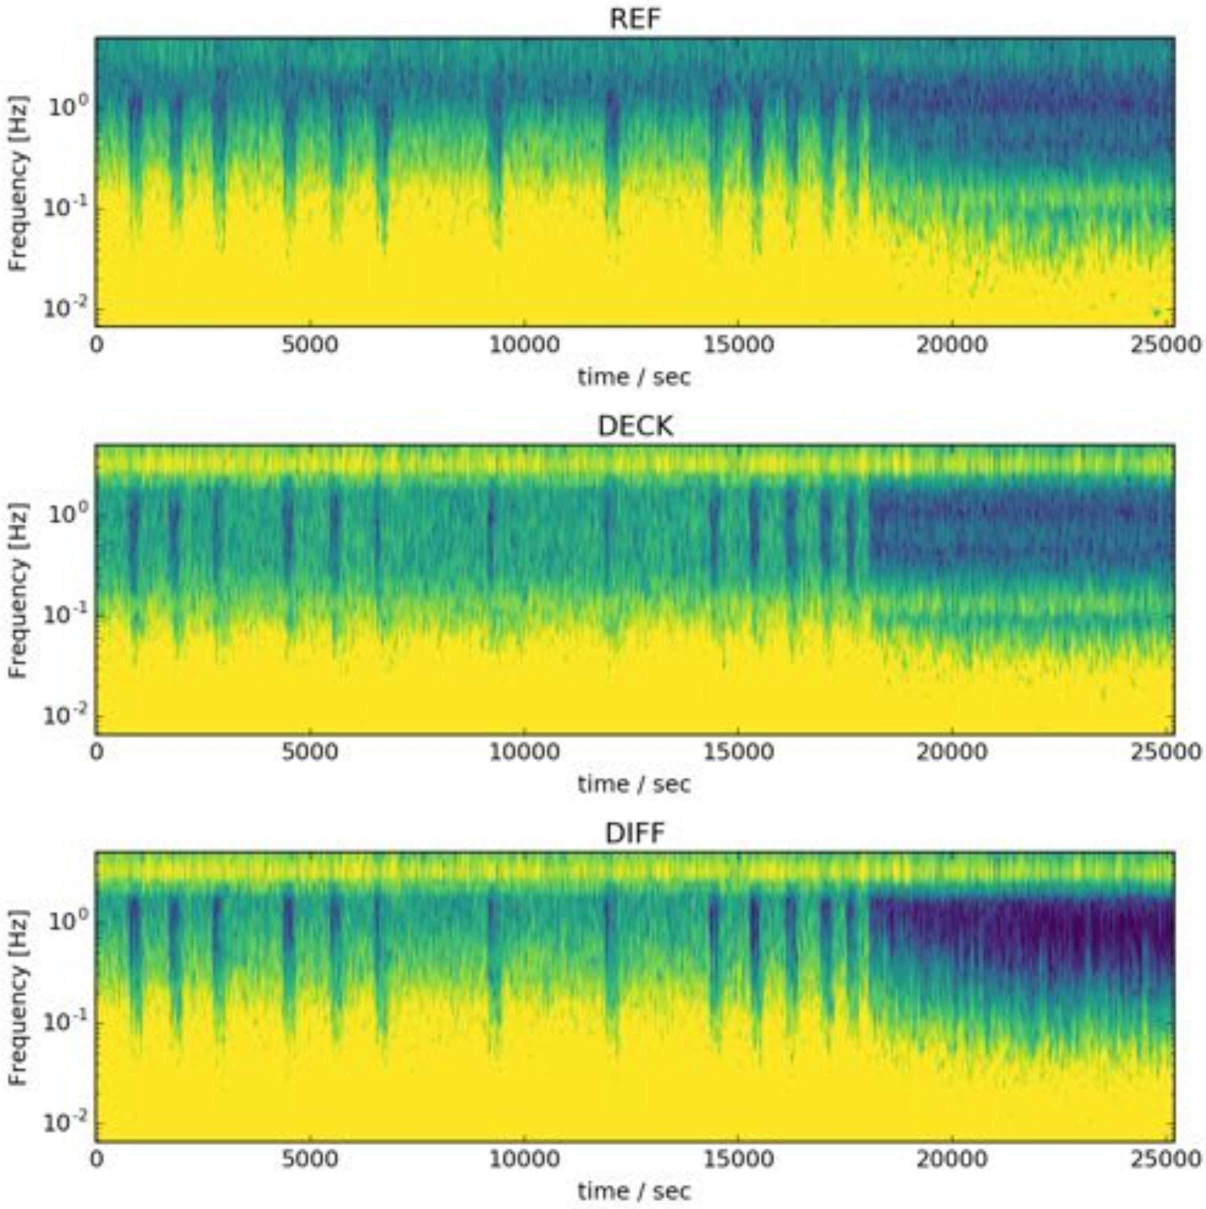


Figure S2: Same as figure S1, for the north component.

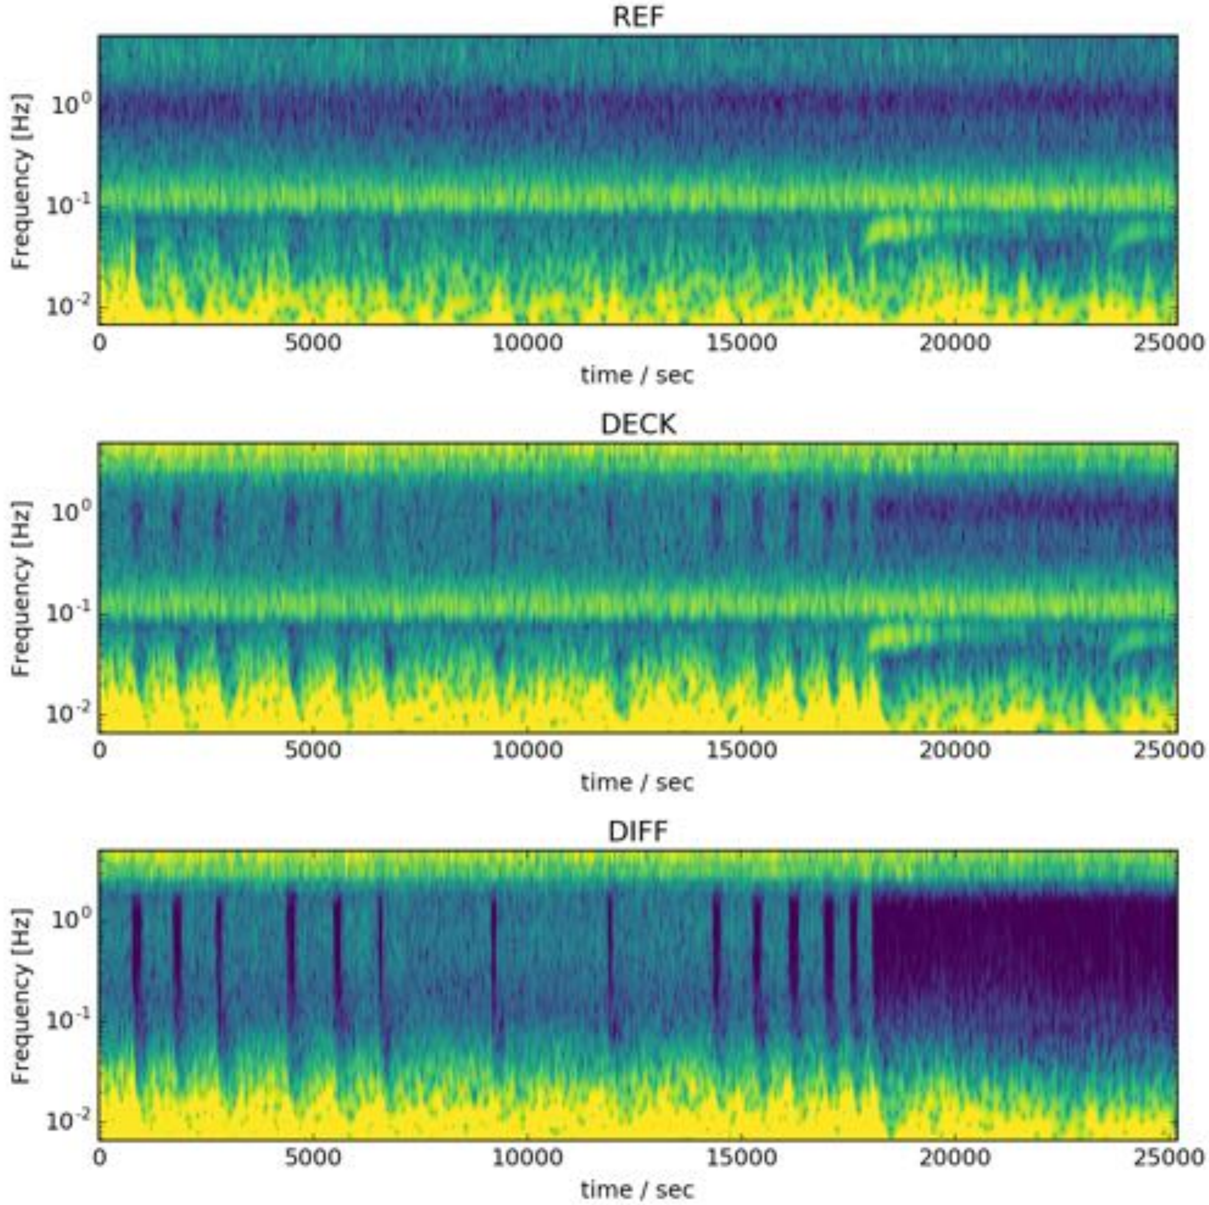


Figure S3: Same as figure S1, for the vertical component.

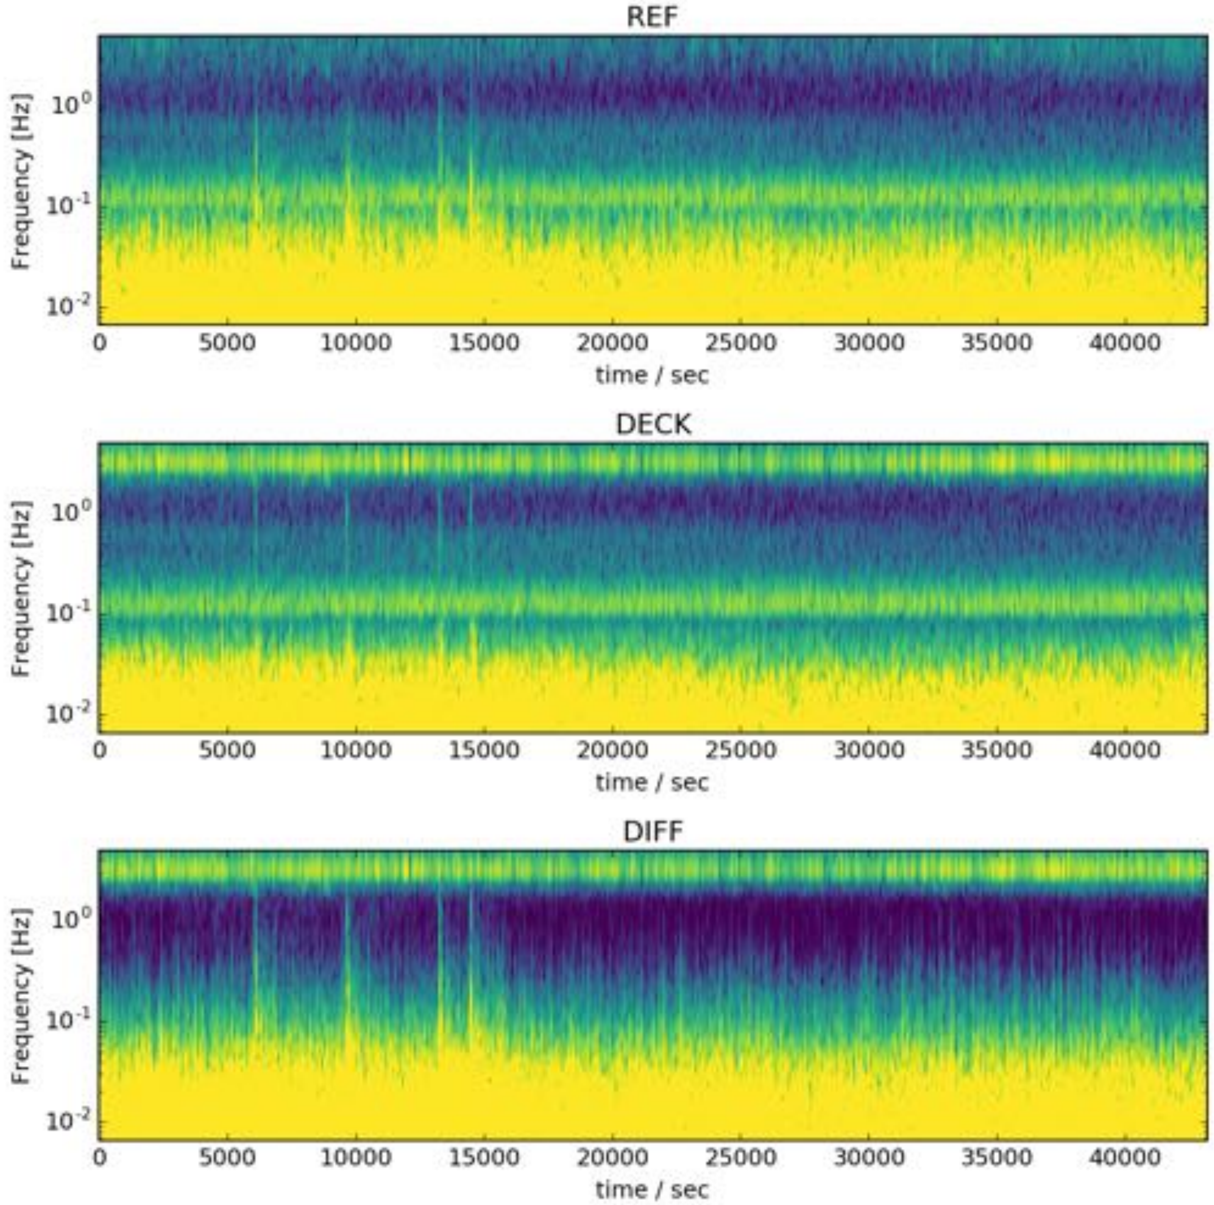


Figure S4: Same as figure S1, but for the east component for the 12-hour period beginning at 2017-10-07 03:00 UTC.

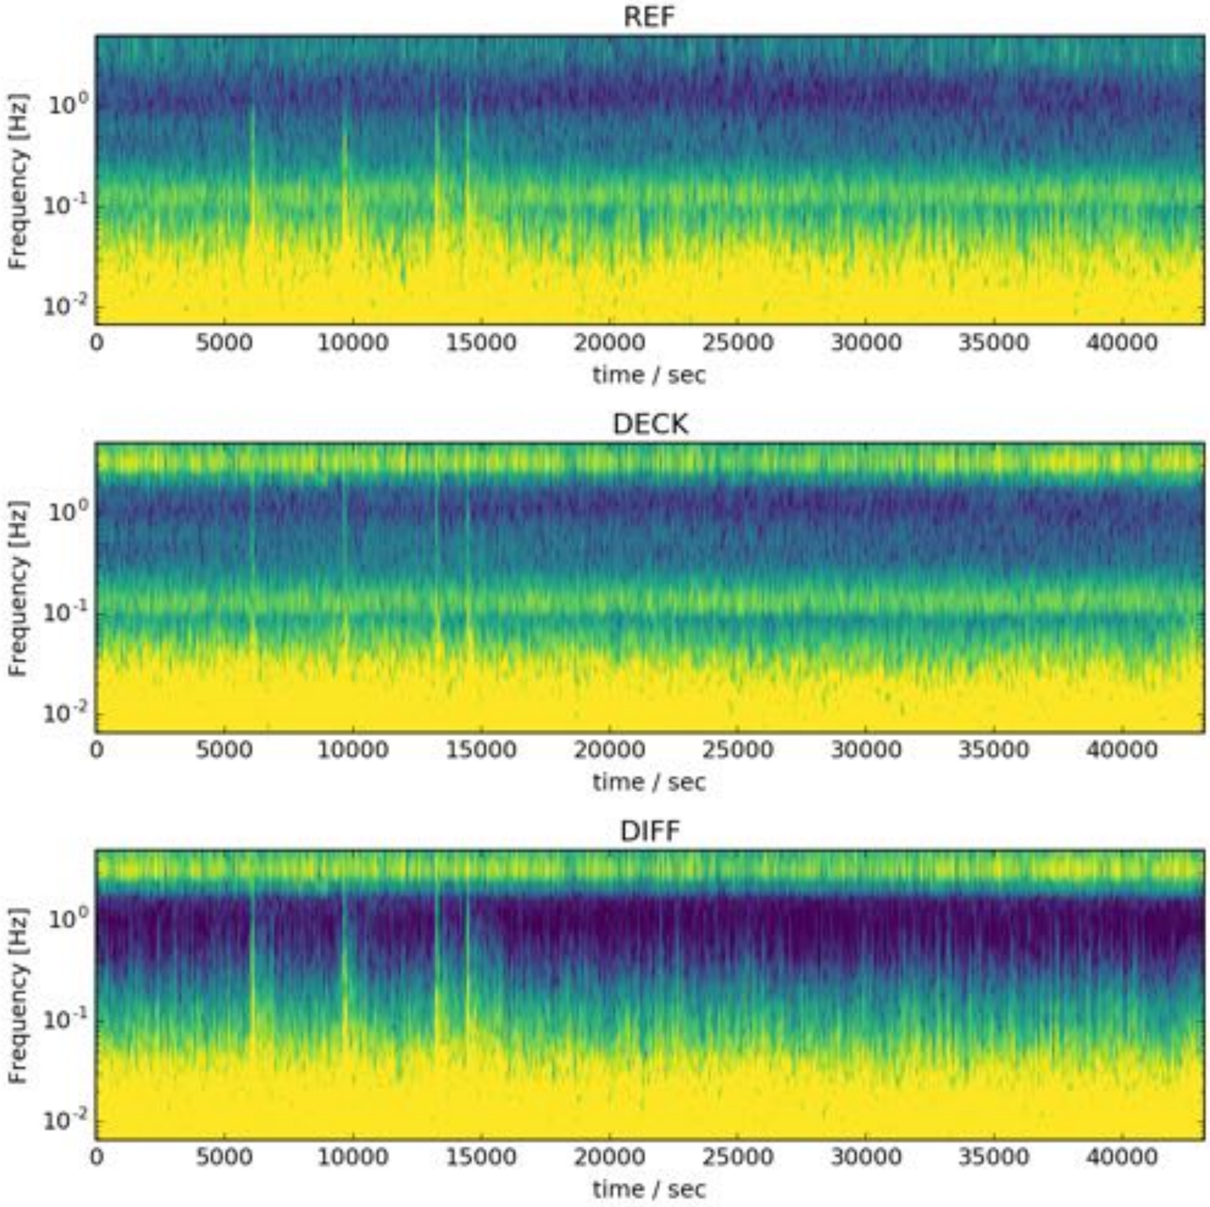


Figure S5: Same as figure S4, but for the north component.

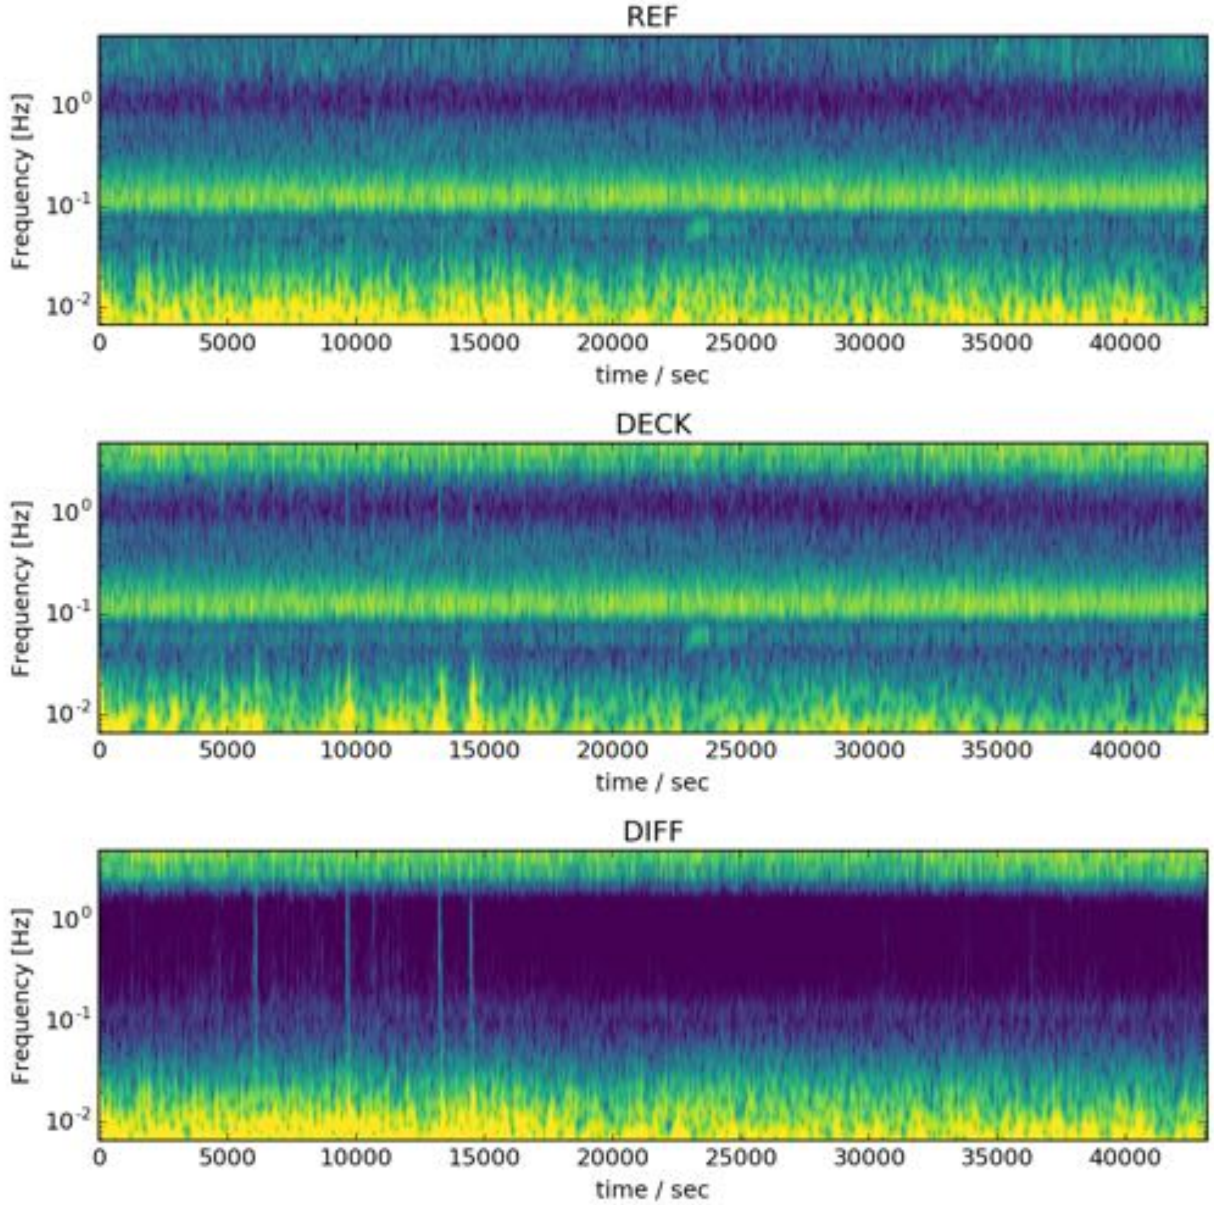


Figure S6: Same as figure S4, but for the vertical component.

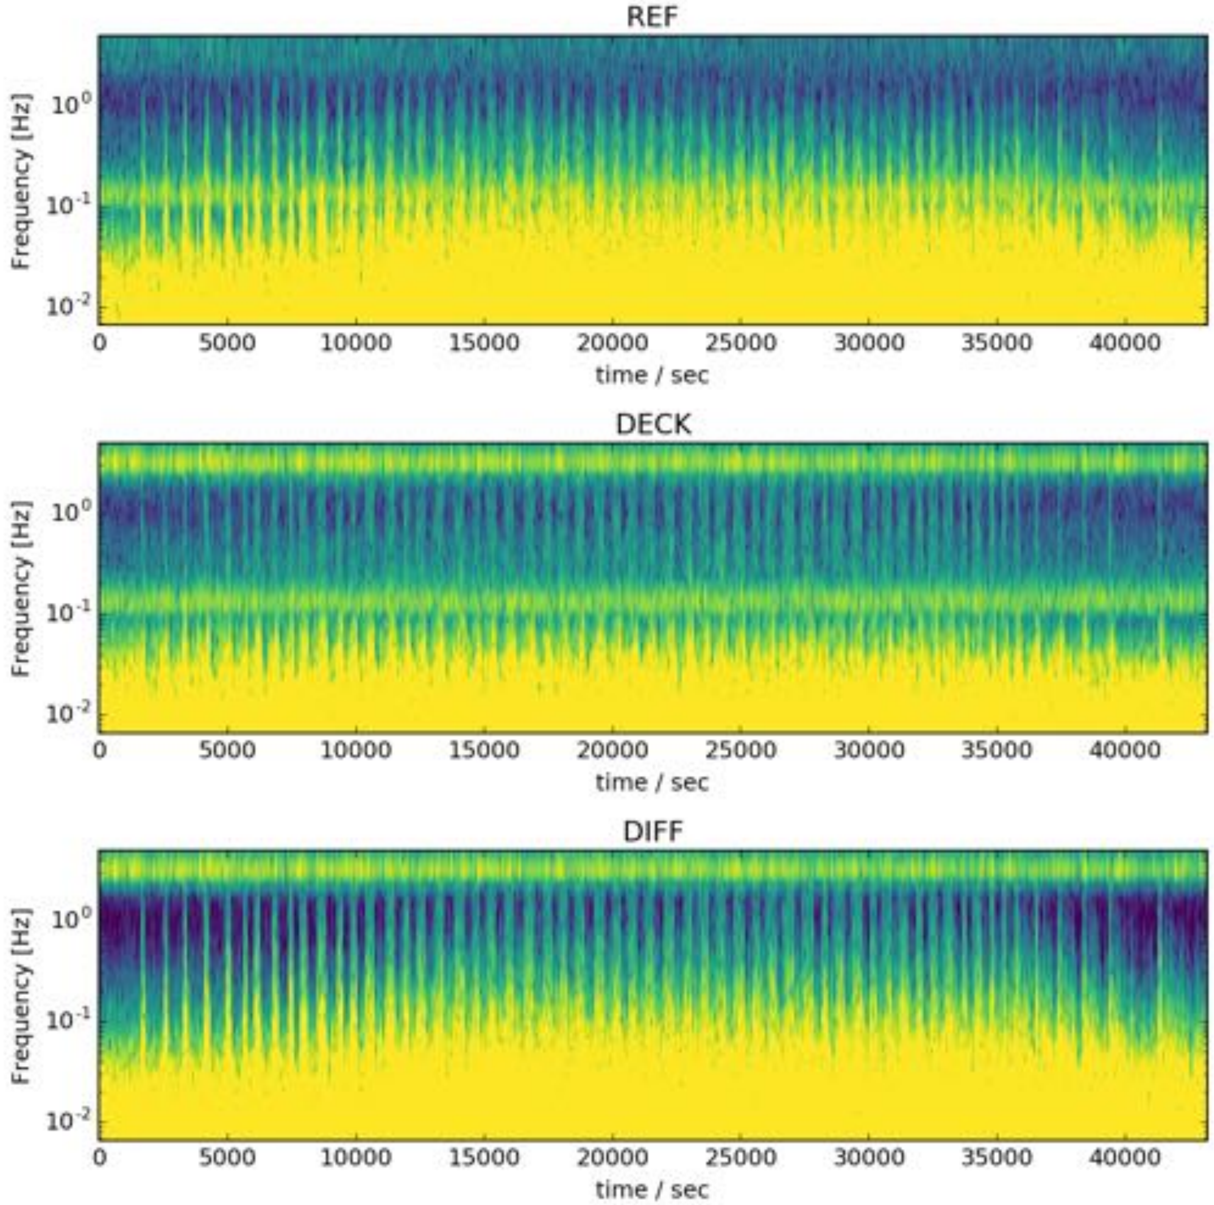


Figure S7: Same as figure S1, but for the east component for the 12-hour period beginning at 2017-10-07 15:00 UTC.

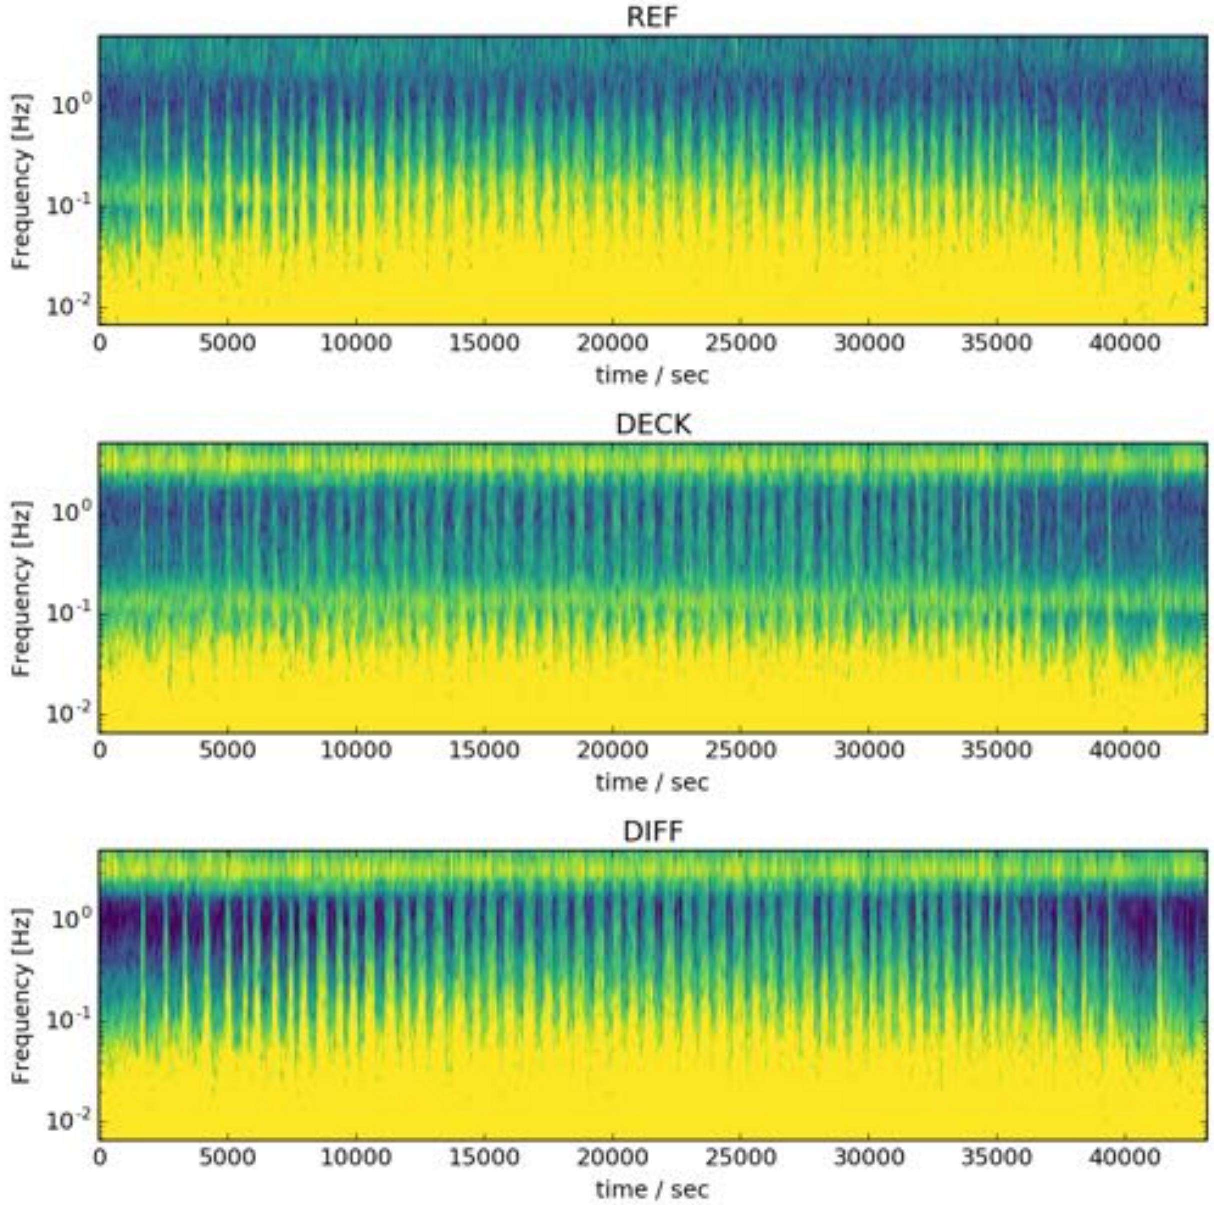


Figure S8: Same as figure S7, but for the north component.

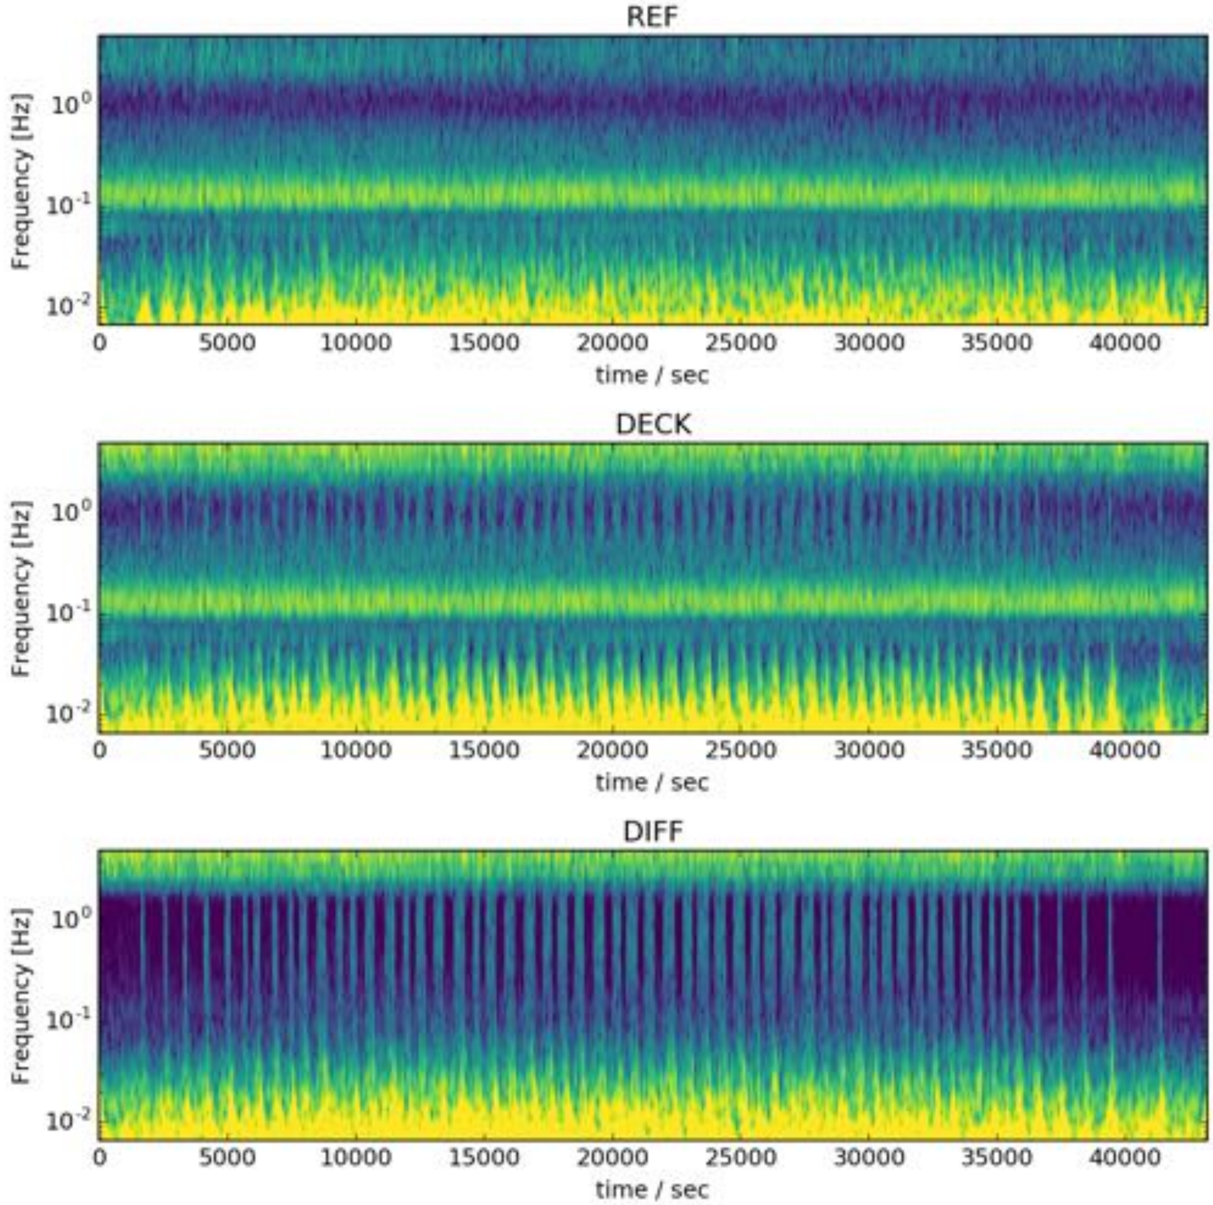


Figure S9: Same as figure S7, but for the vertical component.

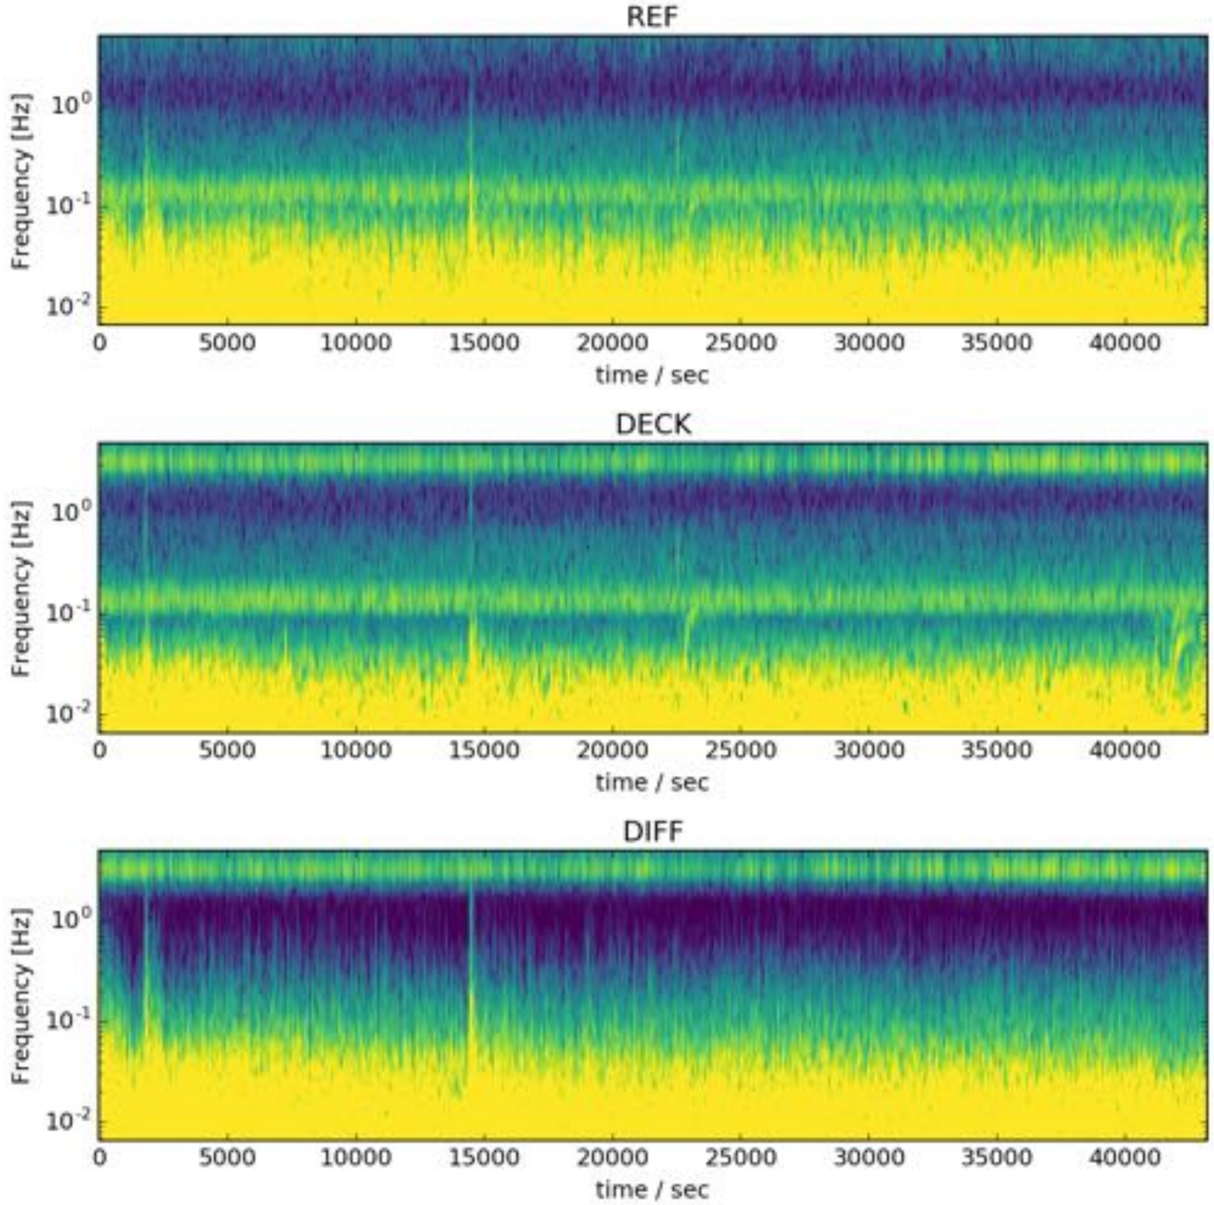


Figure S10: Same as figure S1, but for the east component for the 12-hour time period beginning at 2017-10-08 03:00 UTC.

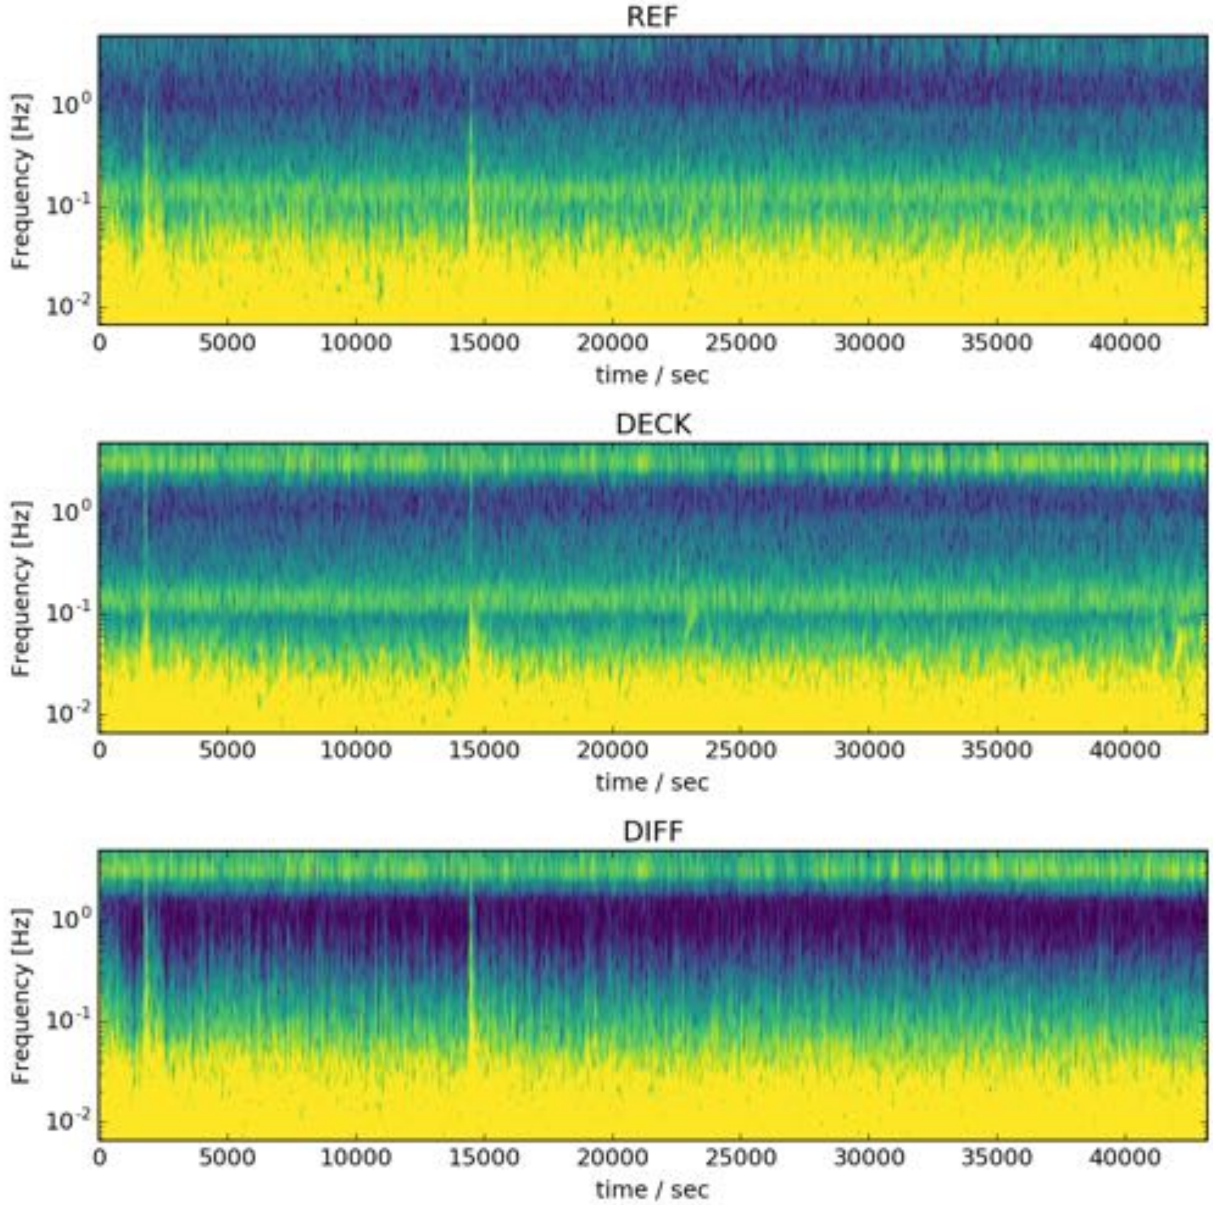


Figure S11: Same as figure S10, but for the north component.

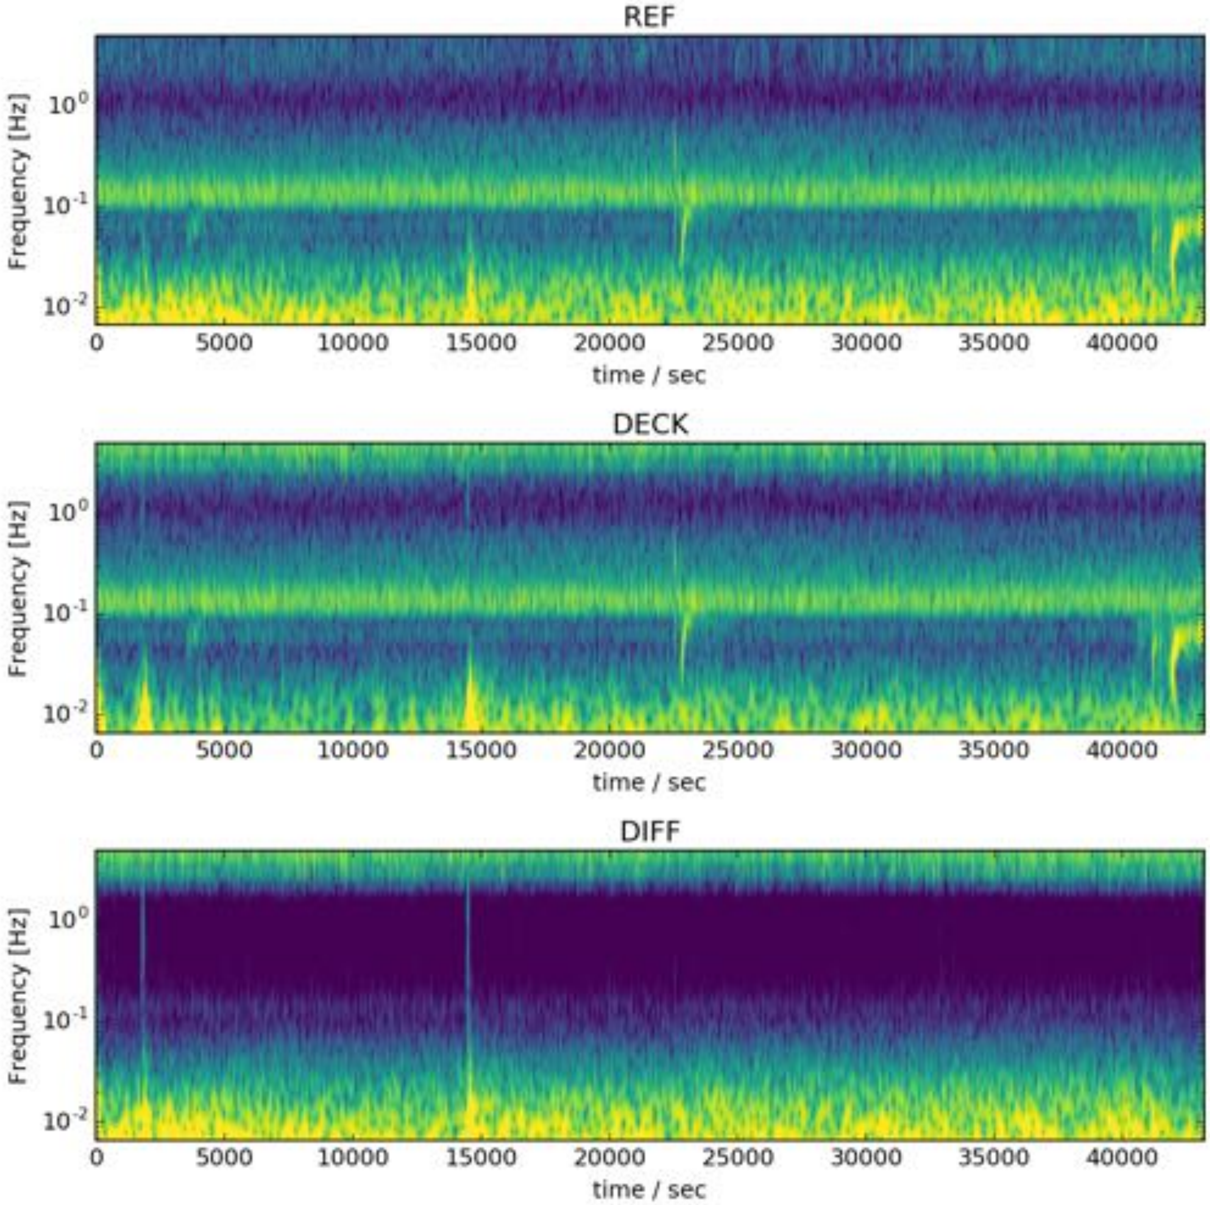


Figure S12: Same as figure S10, but for the vertical component.

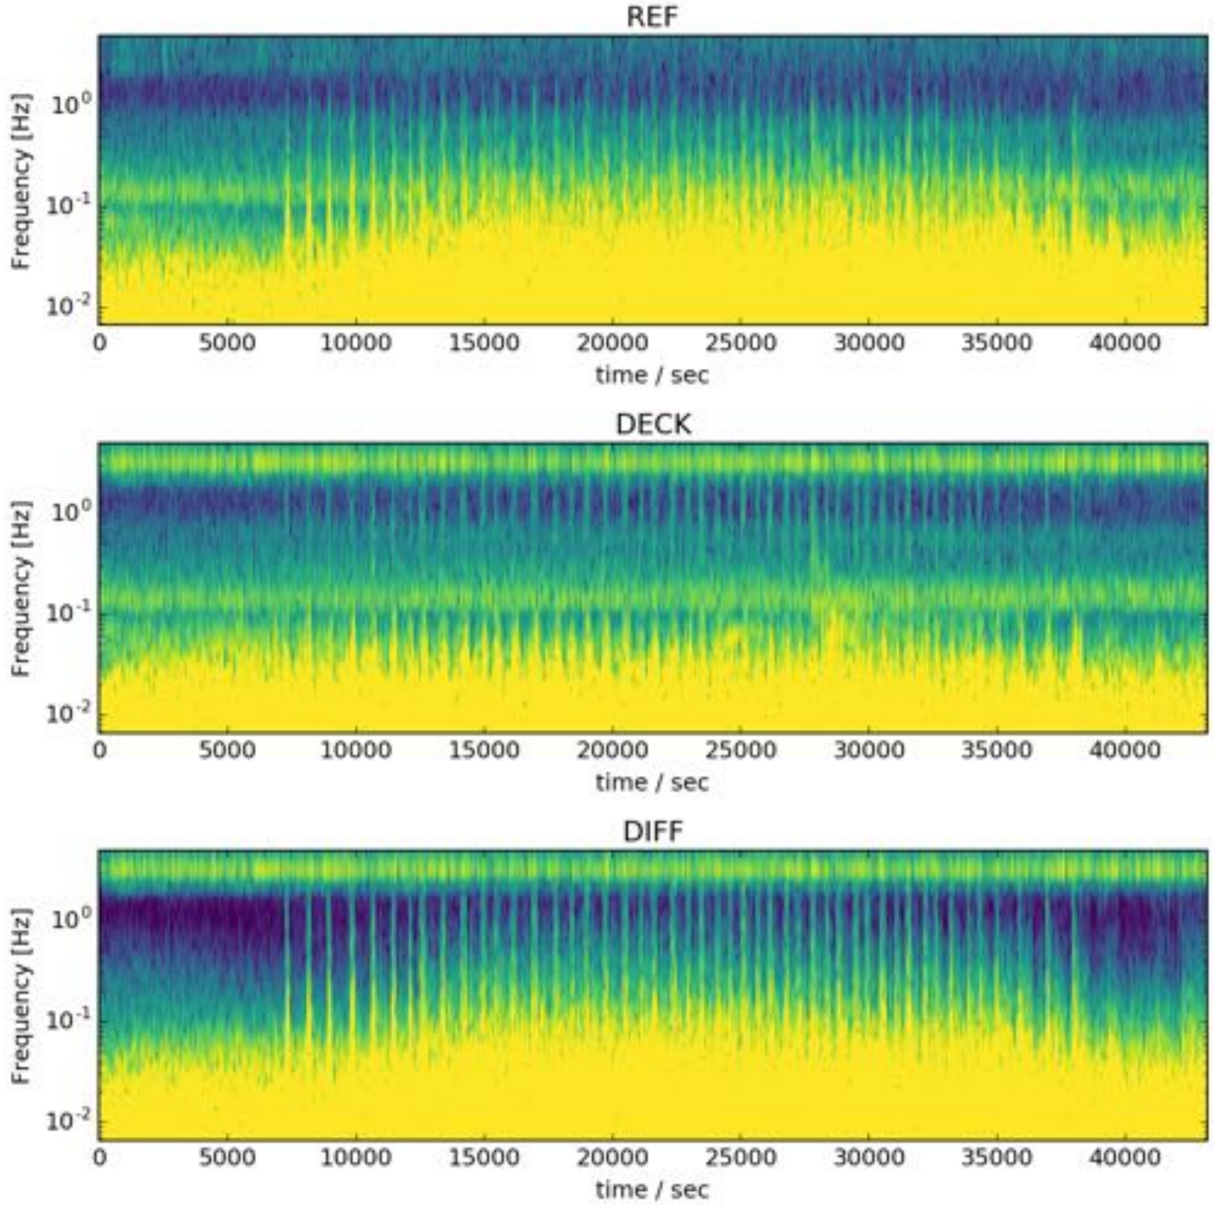


Figure S13: Same as figure S1, but for the east component for the 12-hour period beginning at 2017-10-08 15:00 UTC.

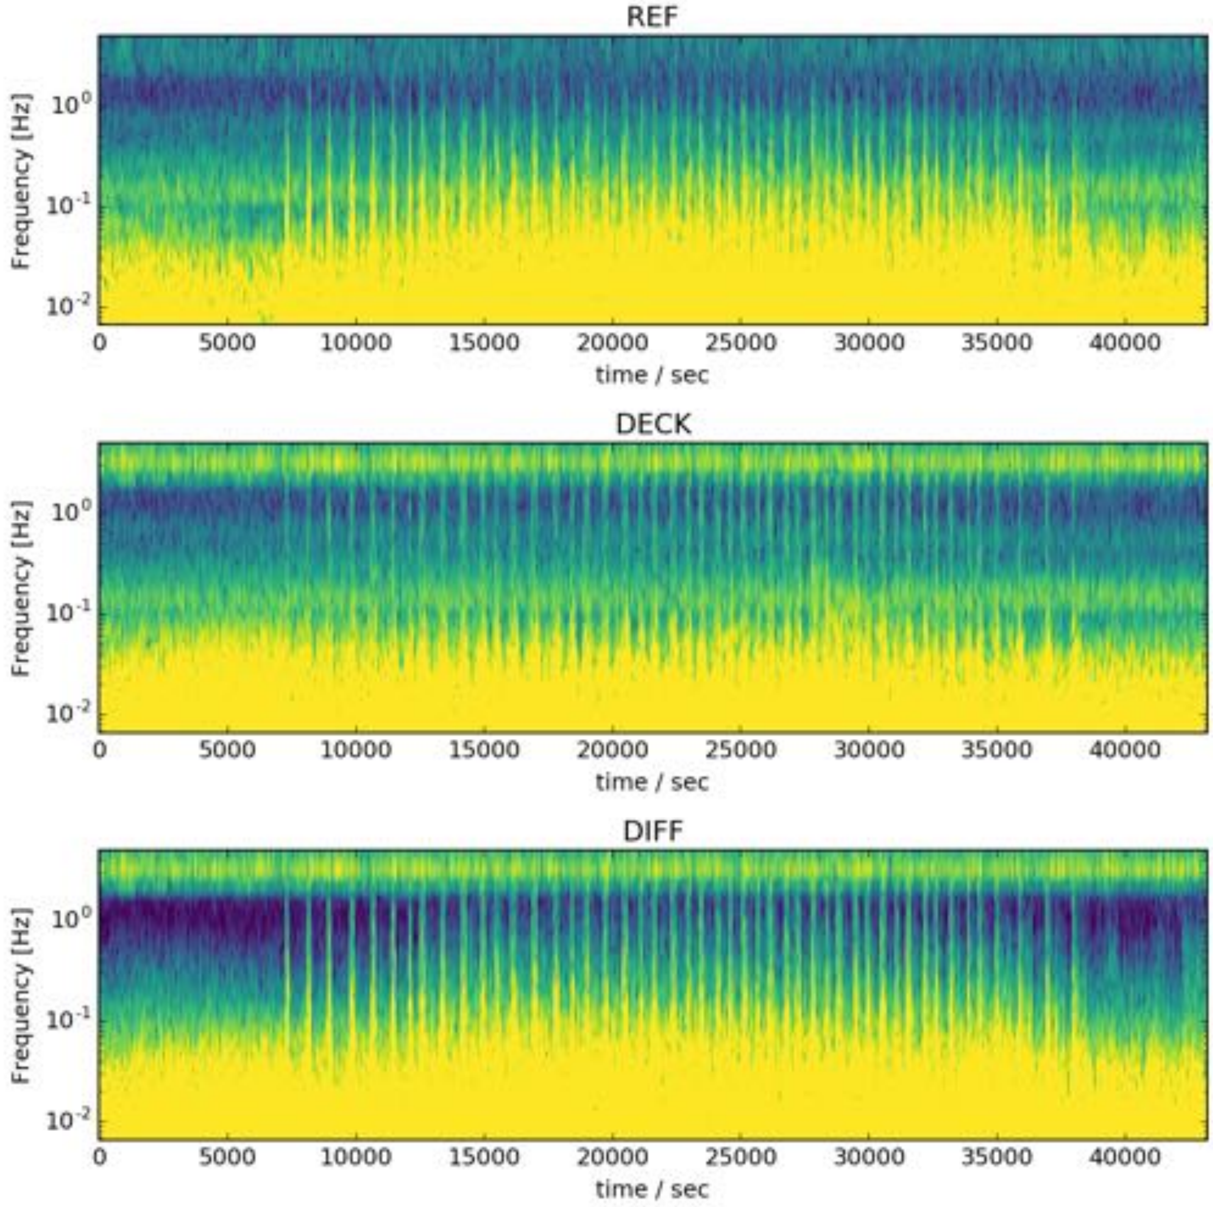


Figure S14: Same as figure S13, but for the north component.

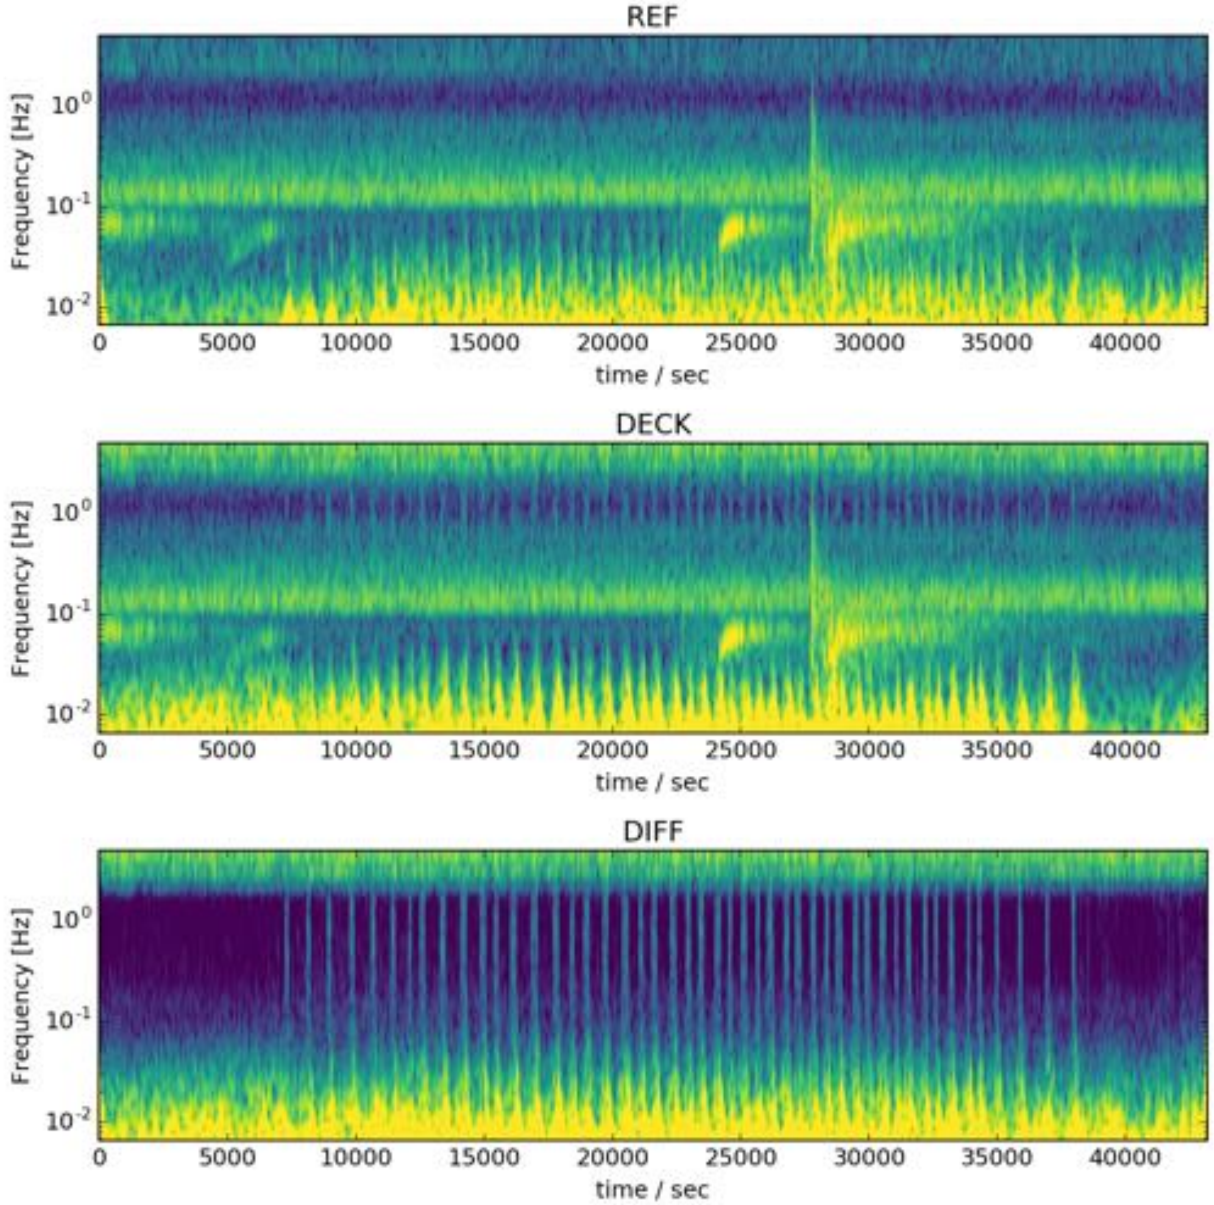


Figure S15: Same as figure S13, but for the vertical component.

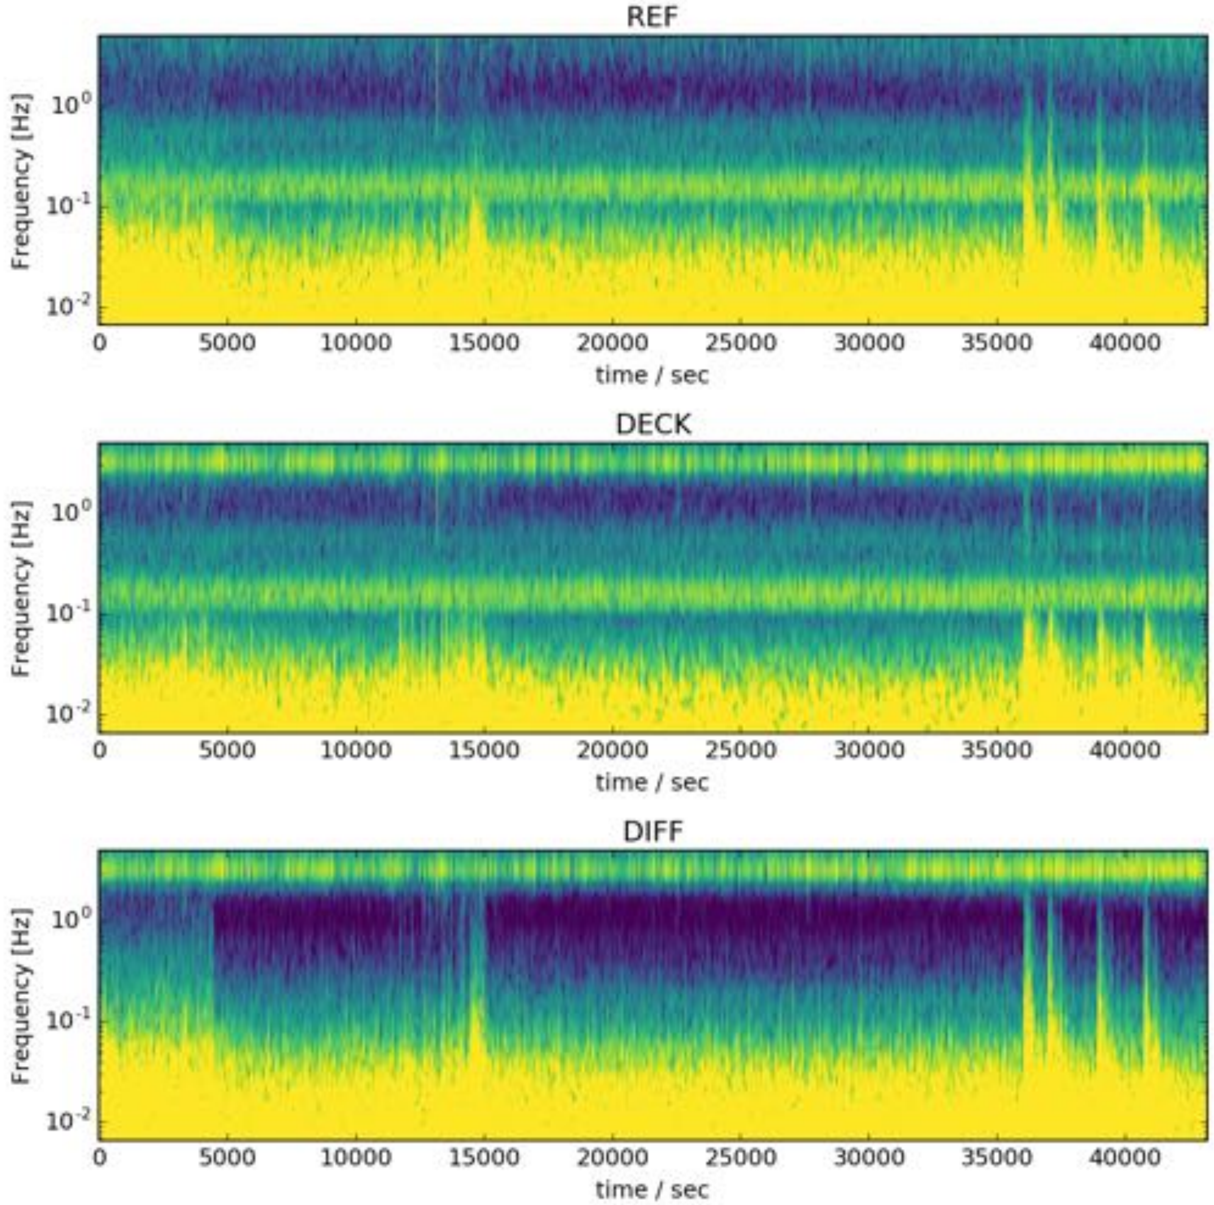


Figure S16: Same as figure S1, but for the east component for the 12-hour period beginning at 2017-10-09 03:00 UTC.

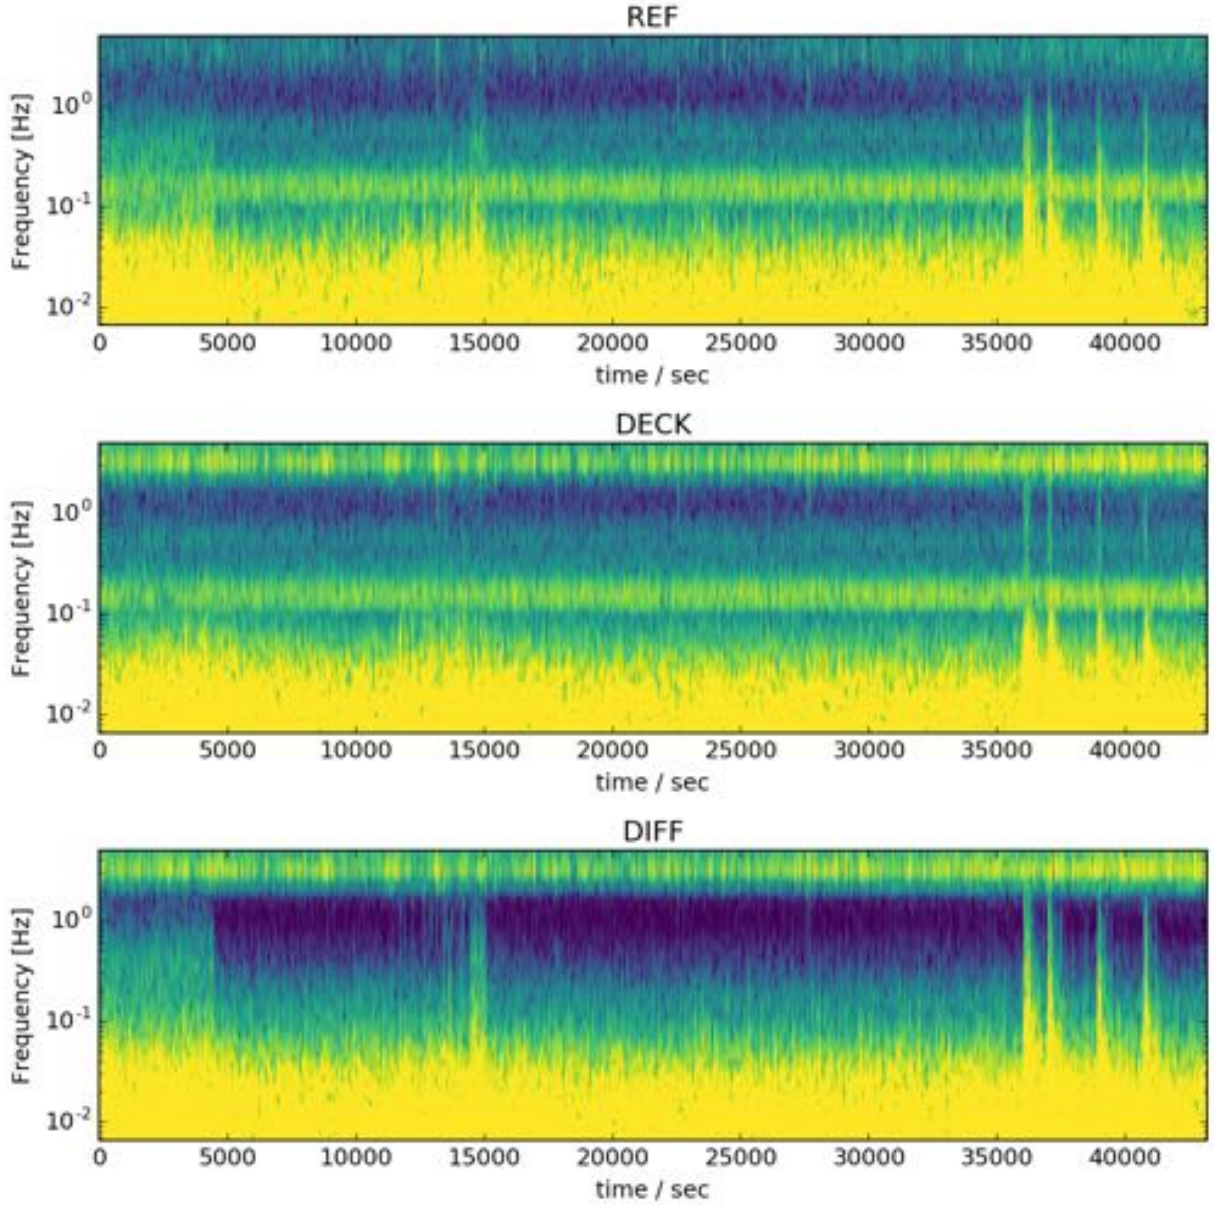


Figure S17: Same as figure S16, but for the north component.

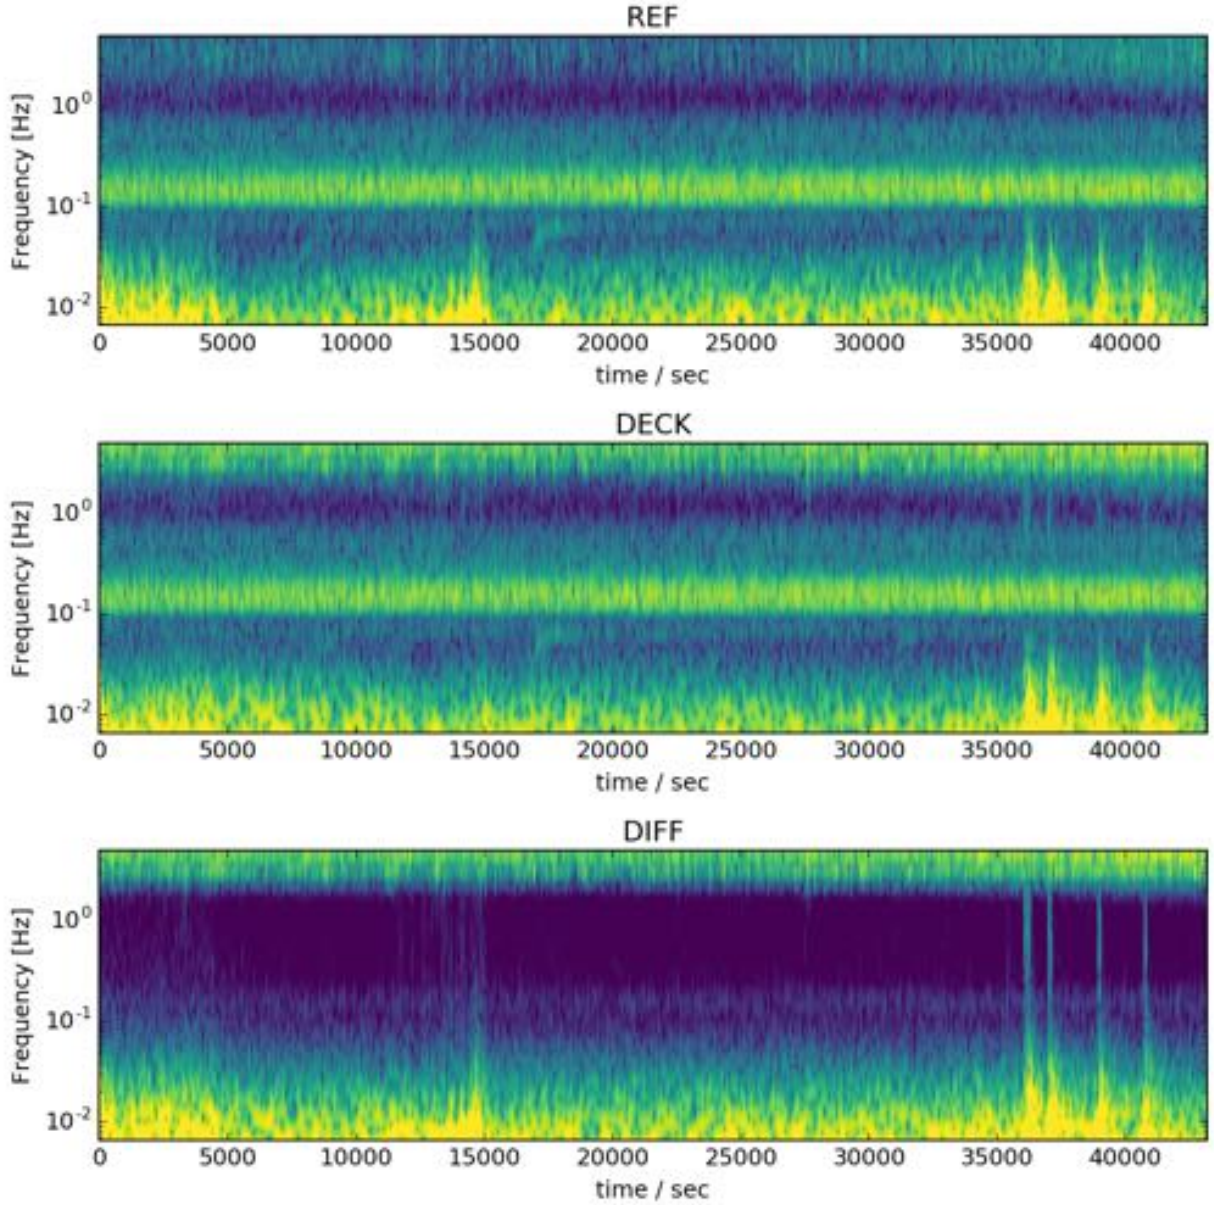


Figure S18: Same as figure S16, but for the vertical component.

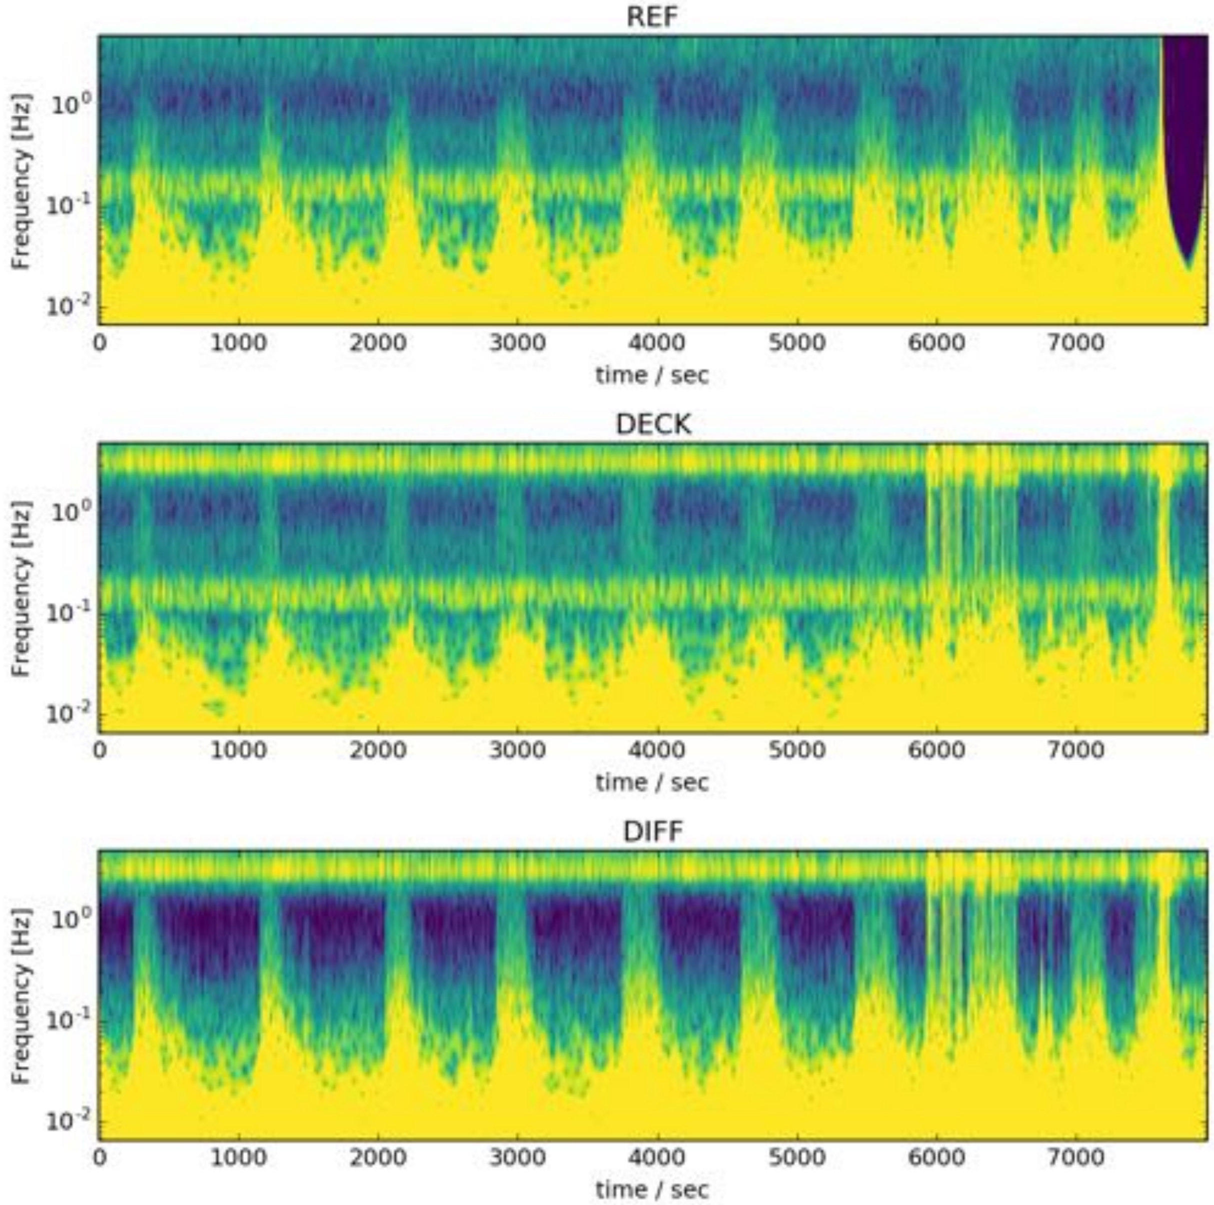


Figure S19: Same as figure S1, but for the east component for the time period from 2017-10-09 15:00 UTC to 2017-10-09 17:12:20 UTC.

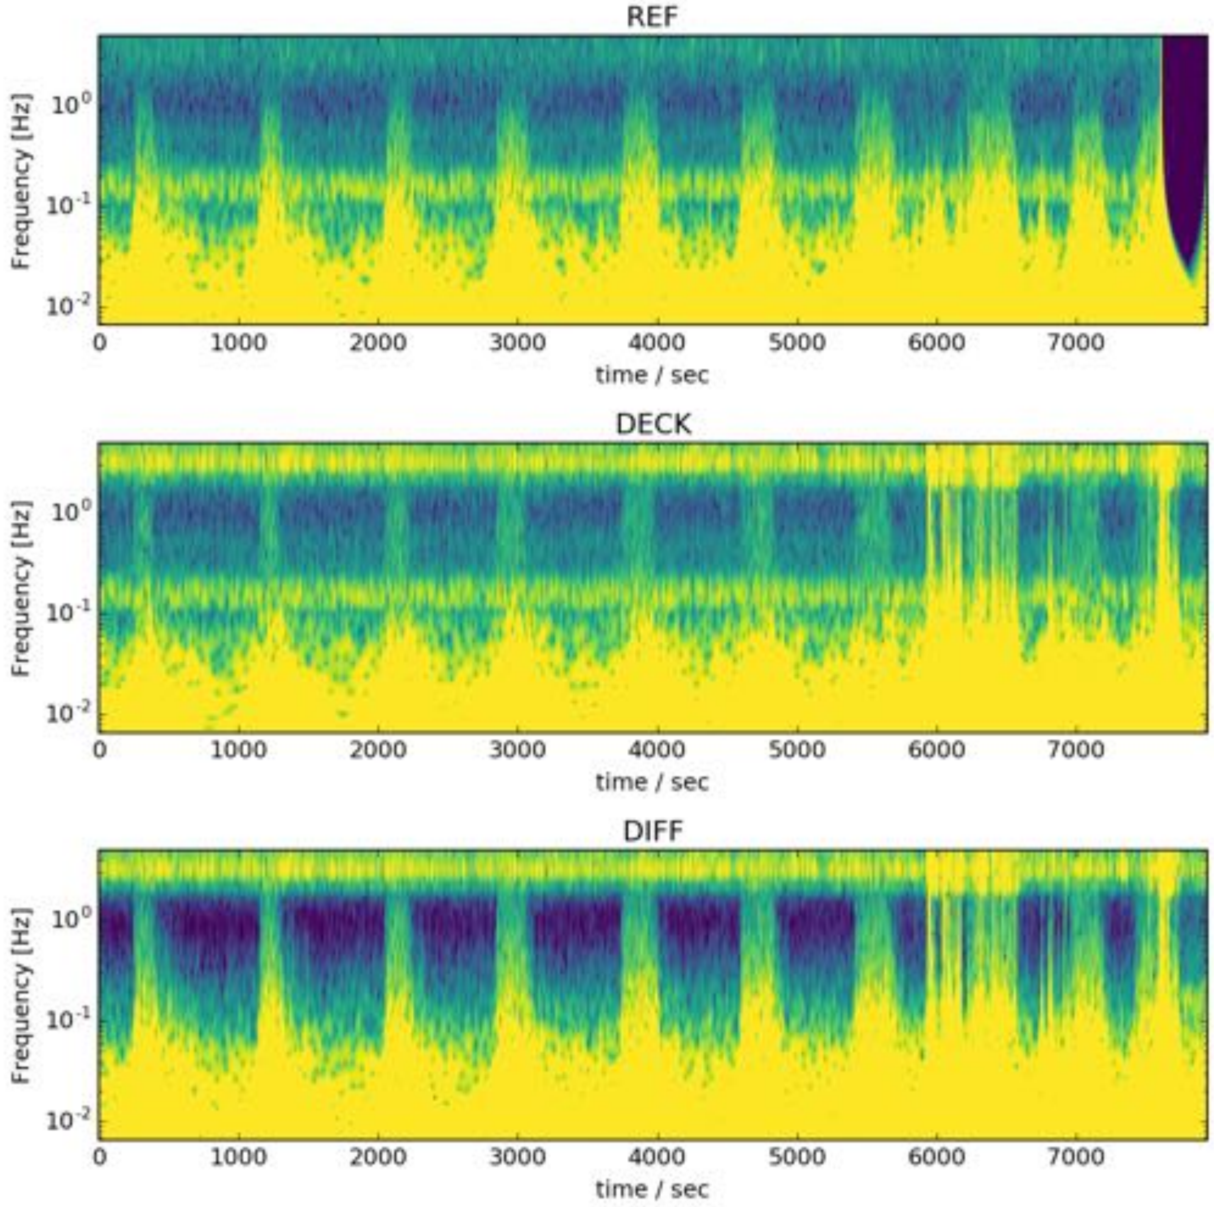


Figure S20: Same as figure S19, but for the north component.

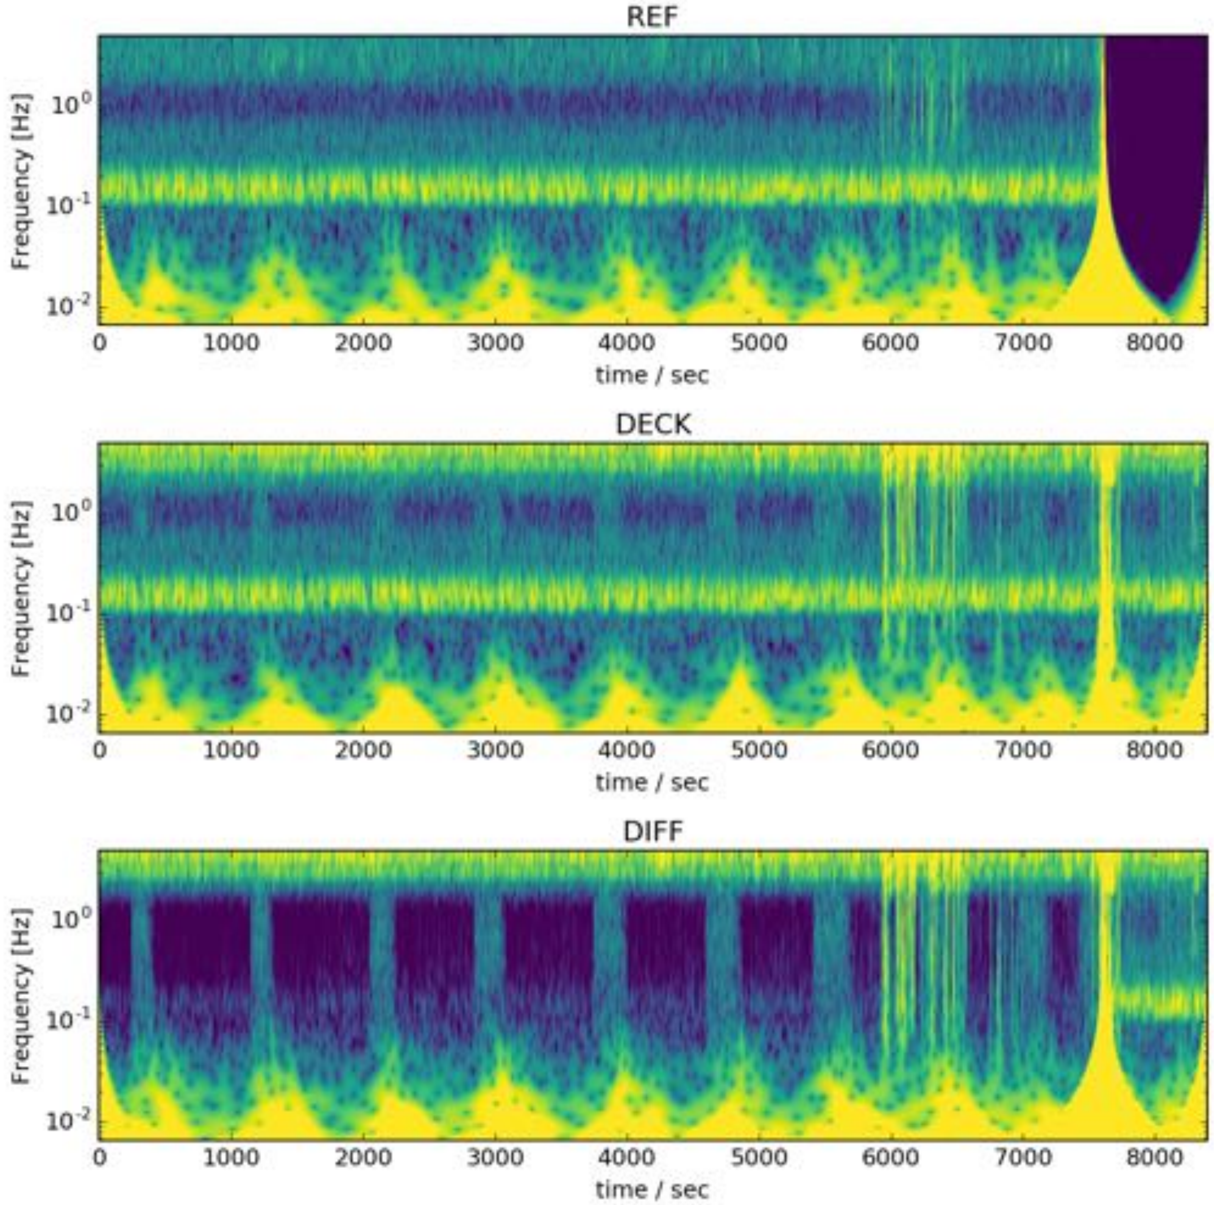


Figure S21: Same as figure S19, but for the vertical component.
